# Supplementary material for: Universal map of gas-dependent kinetic selectivity in carbon nanotube growth
Source: arXiv:2111.08411 ancillary file (2021-11-16)
Supplement: Supplementary file 1 [file growth-kinetics-SI.pdf]

**Supplementary information for**

# Universal map of gas-dependent kinetic selectivity in carbon nanotube growth

Keigo Otsuka,[1,2]* Ryoya Ishimaru,[1] Akari Kobayashi,[1] Taiki Inoue,[3] Rong Xiang,[1] Shohei Chiashi,[1] Yuichiro K. Kato,[2,4] Shigeo Maruyama[1*]

[1] Department of Mechanical Engineering, The University of Tokyo, Tokyo, 113-8656, Japan

[2] Nanoscale Quantum Photonics Laboratory, RIKEN Cluster for Pioneering Research, Saitama, 351-0198, Japan

[3] Department of Applied Physics, Osaka University, Osaka, 565-0871, Japan

[4] Quantum Optoelectronics Research Team, RIKEN Center for Advanced Photonics, Saitama, 351-0198, Japan.

**This PDF file includes:**

Supplementary Notes 1 to 8
Fig. S1 to S15
Table S1 to S3
References

————

* email: otsuka@photon.t.u-tokyo.ac.jp, maruyama@photon.t.u-tokyo.ac.jp

**Supplementary information**

## Supplementary Note 1:

In the Raman mapping image (Fig. 2b), isotope labels colored in blue and green, which correspond to the G-band peaks appearing at ~1580 and ~1568 $cm^{-1}$, respectively, are grown from the mixture of $^{13}C$ ethanol and $^{12}C$ acetylene, while those in red originate dominantly from $^{13}C$ ethanol. A greater number of red labels (#1–3) are found near the catalyst line, which implies that the growth of many nanotubes initiates before the acetylene addition but quickly terminates when too much carbon is supplied from acetylene. Furthermore, when focusing on the incubation time of nanotube growth, we find no SWCNT initiating the growth after the addition of acetylene. Note that in the normal ethanol CVD process without the modulation in conditions, the growth incubation time has a wide distribution including ~0 min and >20 min[1]. This suggests that the high $P_C$ increased by acetylene is not favorable both for nucleation and long-time growth, though the tube chirality and the D/G ratio of Raman spectra is homogeneous along each nanotube as long as the growth continues (Fig. S6).

## Supplementary Note 2:

In Fig. S3, we consider the following gas species arising from ethanol decomposition: $C_2H_5OH$, $C_2H_4$, $H_2O$, $C_2H_2$, $CH_4$, $H_2$, $CO_2$, CO $CH_2$, $C_3H_6$, $CH_3HCO$. These gas species are diluted in an Ar buffer gas. Calculation is performed using the software package COMSOL, based on the kinetic model proposed by N. M. Marinov[2,3]. According to the experimental measurements, the temperature profile along the gas flow has a quadratic temperature distribution at the entrance of the furnace (0–15 cm), while and the temperature at middle (15–45 cm) is the same as the set temperature of the furnace. We assume the flow velocity of 0.125 m/s under the total pressure of 1.3 kPa including the Ar buffer gas.

## Supplementary Note 3:

In order to visualize aligned SWCNTs, we use optical imaging, in which the contrast of nanotubes is enhanced by the nearly crossed polarizers[4]. LED light goes through a Glan-Thompson polarizer (Thorlabs, GTH10) and an objective (Olympus, MPLFLN50XBDP), and then illuminates nanotubes oriented at nearly 45 degrees. The effective numerical aperture of the incident light is reduced by an aperture. The reflected light from the sample is collected through the same objective and passes through another Glan-Thompson polarizer nearly crossed with the first one. The images are taken with a commercial camera (Canon, Kiss X10). To further enhance the image contrast and subtract the color of substrates, we perform the following image processing. First, we take an image without LED illumination to acquire a background image $I_{BG}$ (RGB values between 0–255). The image of a bare substrate without nanotubes $I_{ref}$ is then captured as a reference, followed by the acquisition of a nanotube array image $I_{NT}$. With $a$ (<1) and $b$ (>1) being thresholds, the final image $I_P$ is acquired through the following processing for contrast enhancement:

$$I_P = \frac{255}{b-a}\left(\frac{I_{NT}-I_{BG}}{I_{ref}-I_{BG}} - a\right). \tag{S1}$$

A typical value for a (b) is 0.89 (1.19) for red and green, but 0.94 (1.11) for blue due to a small extinction ratio of the polarizers for short wavelengths. We automatically acquire and process hundreds of images, and then form an image in a large area by joining them together. A typical image at a selected area is shown in Fig. S15.

**Supplementary information**

## Supplementary Note 4:

In the proposed kinetic model, we assume all the rates ($\Gamma_e$, $\Gamma_C$, and $\gamma_g$) are in a linear regime by considering only a small shift from an equilibrium state (Fig. 1d). For example, the adsorption rate $\Gamma_C$ would be saturated, i.e., effective surface area of the catalyst decreases, as $P_C$ and correspondingly $N$ (or coverage of catalyst surface by carbon) increase. The extreme case of increased coverage should be the growth termination due to encapsulation of the catalyst. We note that such a saturation effect in carbon adsorption rates cannot explain the deviation between a $P_C$ multiplication factor and growth acceleration $\gamma_{g,2}/\gamma_{g,1}$; it would rather result in $\gamma_{g,2}/\gamma_{g,1} < \lambda$, which contradicts the experimental observations.

For the adsorption of carbon atoms from precursors, we consider single values for the kinetic constant $k_{ad}$ and the carbon source pressure $P_C$ for simplicity. More precisely, when multiple types of carbon sources with different adsorption efficiencies, the adsorption rate of carbon atoms should be $\Gamma_C = \sum_i Ak_{\mathrm{ad},i}P_{\mathrm{C},i} = Ak_{\mathrm{ad}}P_{\mathrm{C}}$, where $i$ represents different carbon-containing molecules.

## Supplementary Note 5:

To explain the experimental relationship between $\gamma_{g,1}$ and $\gamma_{g,2}$ (Fig. 2d), other parameters than $k_e$ can be eliminated. When assuming the variation in $k_g$ or $D'$ (=$D/A$) accounts for the growth rate variation, we can derive the following equation:

$$\gamma_{\mathrm{g},2} = \frac{\lambda k_{\mathrm{ad}}P_{\mathrm{C}} - k_{\mathrm{e}}N_{\mathrm{eq}}P_{\mathrm{e}}}{k_{\mathrm{ad}}P_{\mathrm{C}} - k_{\mathrm{e}}N_{\mathrm{eq}}P_{\mathrm{e}}}\gamma_{\mathrm{g},1}, \tag{S2}$$

where $\gamma_{g,2}$ should approach 0 at the limit of $\gamma_{g,1}$=0. Also, the slope would be > $\lambda$. In these senses, this equation is inconsistent with the experimental results. On the other hand, if we consider $N_{eq}$ to be the dominant factor that determine the growth rate, we can link $\gamma_{g,1}$ and $\gamma_{g,2}$ by the equation below:

$$\gamma_{\mathrm{g},2} = \gamma_{\mathrm{g},1} + \frac{k_{\mathrm{ad}}P_{\mathrm{C}}k_{\mathrm{g}}}{k_{\mathrm{g}}D' + k_{\mathrm{e}}P_{\mathrm{e}}}(\lambda - 1), \tag{S3}$$

In this case, the slope should be 1 regardless of $\lambda$, but it is also inconsistent with the experiments where the slopes of 1.7 and 1.8 are obtained for $\gamma_{g,2}$ and $\gamma_{g,3}$, respectively.

The removal rate $\Gamma_e$ of carbon from the catalyst nanoparticles is given by,

$$\Gamma_{\mathrm{e}} = Ak_{\mathrm{e}}P_{\mathrm{e}}(\Delta N + N_{\mathrm{eq}}) = Ak_{\mathrm{e}}P_{\mathrm{e}}\frac{k_{\mathrm{ad}}P_{\mathrm{C}} + k_{\mathrm{g}}D'N_{\mathrm{eq}}}{k_{\mathrm{g}}D' + k_{\mathrm{e}}P_{\mathrm{e}}}. \tag{S4}$$

Hence, when $P_C$ is increased from $P_C$ to $\lambda P_C$, we define the multiplication factor $s$ for the removal rate by $\Gamma_e(\lambda P_C)/\Gamma_e(P_C)$ (=$N_2/N_1$) as shown in the main text as well. As we find that $k_e$ is the key parameter that accounts for the tube-to-tube $\gamma_g$ variance, $s$ can be obtained from the slope of $\gamma_{g,1}$-$\gamma_{g,2}$ relationships (Fig. 2d), allowing for the estimation of $\Gamma_C$ and $\Gamma_e$ for each nanotube by Eq. 4 and 5 in the main text.

When adding acetylene with two different flow rates, the $P_C$ multiplication factor $\lambda$ are 2.39 and 3.28. The corresponding $\gamma_{g,1}$- $\gamma_{g,2}$ relationships give the y-intercepts of 14.4 and 23.0 μm/min, the ratio of which agrees to that of $\lambda - 1$. The agreement of these pairs of numbers (see Eq. 6 in the main text) derived from different aspects of measurements, namely G-mode downshifts by $^{13}C$ mixture and distance between isotope labels, is consistent with the assumption made for Eq. 6 or Eq. S3.

## Supplementary Note 6:

The $^{12}C$ content in the isotope label #5 varies tube to tube likely depending on the metallicity as well, and the variance may arise from the different adsorption efficiency of carbon sources to the catalyst. By assuming that acetylene originates from the additive acetylene or the decomposition of ethanol, we consider $k_{ad}$ for acetylene and other carbon sources (ethanol, ethylene, etc.). The partial pressure of $^{13}C$ acetylene $P_{ac,13}$ that originates from $^{13}C$ ethanol is experimentally unknown but can be estimated from the simulations on ethanol decomposition (Fig. S3), whereas that of $^{12}C$ acetylene $P_{ac,12}$ is 1.9 Pa according to the flow rate comparison. The dominant product of ethanol decomposition are ethylene and water, but only ethylene is incorporated into CNTs. By taking the number of carbon atoms into account, the total pressure of ethanol and ethylene $P_{et,13}$ in the furnace should be almost equal to the initial ethanol pressure, and we take $P_{et,13}$ to be 122 Pa. With $k_{ad,ac}$ and $k_{ad,et}$ being the adsorption efficiency of acetylene and the average of ethanol and ethylene, we obtain the following equation for $\alpha$:

$$\alpha = \frac{P_{ac,12}R}{P_{et,13} + (P_{ac,13} + p_{ac,12})R}, \qquad \text{(S5)}$$

where $R = k_{ad,ac}/k_{ad,et}$. Fig. S8c shows $\alpha$ as a function of $R$ and $P_{ac,13}$, unknown parameters in the experiments. Note that $P_{ac,13}$ should be the same of all nanotubes within a substrate, while $R$ should be different for each catalyst-nanotube pair. If we assume $P_{ac,13}$ to be 0.1 Pa according to Fig. S3, the relationship between $\alpha$ and $R$ can be reduced to Fig. S8d.

## Supplementary Note 7:

In the isotope labeling experiment that shown in Fig. 3f–h, the peak frequency of G and D modes can be converted to the time when the corresponding part of a nanotube are grown. The fraction of $^{13}C$ ethanol $\beta$ is a function of time and expressed as $\beta = t/180$, where $t$ [s] represents the time after the ethanol supply starts. When ethanol with $^{13}C$ fraction of $\beta$ is supplied to catalysts, the corresponding G peak $\omega_G$ of nanotubes will be $\omega_G = \omega_0\sqrt{12.01/\,(12.01(1-\beta) + 12.99\beta)}$, and we assume $\omega_0$=1595 cm$^{-1}$ for all nanotubes based on the experiments in Fig. 2. The linear approximation of the $t$- $\omega_G$ relationship becomes $t = -2.916\omega_G + 4716$ [s] for the G mode, and $t = -3.511\omega_D + 4686$ [s] for the D mode ($\omega_D$). We can obtain the growth rate $dx/dt$ from the slope in Fig. 3g ($d\omega_G/dx$) and $dt/d\omega_G$.

## Supplementary Note 8:

Without taking the absolute value of $\gamma_g$, we obtain the analytical expression of the sensitivity of $\gamma_g$ to $k_g$ and $k_e$ using following equations,

$$S_g = \frac{\partial \ln \gamma_g}{\partial \ln k_g} = \frac{k_e P_e}{k_g D' + k_e P_e}, \qquad \text{(S6)}$$

$$S_e = \frac{\partial \ln \gamma_g}{\partial \ln k_e} = -\frac{k_e\left(k_g D' N_{eq} + k_{ad} P_C\right)}{\left(k_g D' + k_e P_e\right)\left(\frac{P_C}{P_e} - \frac{k_e N_{eq}}{k_{ad}}\right)}. \qquad \text{(S7)}$$

As $D'$ and $k_g$ are inherent to the catalyst-nanotube system, $S_g$ monotonically increases and approach 1 at a very large $P_e$. Sensitivity to carbon removal will diverge when $P_C/P_e = N_{eq}k_e/k_{ad}$ but approach zero at a very large $P_C/P_e$. In order to quantitively express the dominance of $k_g$, in determining growth rate, we define $S_{g/e} = S_g + \zeta S_e$. Since the growth rate is always more sensitive

to $k_e$ than to $k_g$ ($|S_e|>|S_g|$), a weight coefficient $\zeta=0.2$ is used to obtain positive $S_{g/e}$ for the conditions where $k_g$-dependent growth rate clearly observed (Fig. 3e (lower panel) and 3h).

**Supplementary information**

**Table S1 | List of variables and constants used in the paper**. Units are given only for ease of understanding, and values used in the analytic model and simulations do not necessarily reflect the actual quantities. The values with asterisk (*) can be different depending on the gas composition, but those corresponding to the low-pressure ethanol CVD and acetylene addition (0.077 sccm) are shown.

| | explanation | (average) values in the model | s.d. in simulation | unit | notes |
|---|---|---|---|---|---|
| $\Gamma_C$ | carbon supply rate | | | $s^{-1}$ | $=A*k_{ad}*P_C$<br>$\gamma_C = \Gamma_C/D$ |
| $\Gamma_e$ | carbon removal rate | | | $s^{-1}$ | $=A*k_e*P_e*N$<br>$\gamma_e = \Gamma_e/D$ |
| $\gamma_g$ | growth rate | | | $nm\cdot s^{-1}$ | $=k_g*\Delta N$ |
| $D$ | number of atoms per unit length<br>(∝ diameter) | 1.00 | | $nm^{-1}$ | With $d$ [nm] being a tube diameter, $D$=120$d$. |
| $N$ | carbon concentration on catalyst | | | $nm^{-3}$ | |
| $N_{eq}$ | carbon concentration at equilibrium | 30 | | $nm^{-3}$ | constant |
| $\Delta N$ | degree of supersaturation | | | $nm^{-3}$ | driving force of growth |
| $A$ | effective surface area of catalyst | 7.07 | 5% | $nm^2$ | Should be smaller than the surface area of nanoparticles because of a tube attached to the catalyst and carbon atoms already dissolved. |
| $k_{ad}$ | adsorption efficiency of carbon | 3.20 | | $nm^{-2}\cdot s^{-1}\cdot Pa^{-1}$ | constant |
| $k_e$ | kinetic constant for carbon removal | 0.054 | 20% | $nm\cdot s^{-1}\cdot Pa^{-1}$ | Dominant at a small $P_e$. |

**Supplementary information**

| | | | | | |
|---|---|---|---|---|---|
| $k_g$ | kinetic constant for growth (shrinkage) | 0.85 | 20% | $nm^4 \cdot s^{-1}$ | dominant at a large $P_e$<br>Probably depending on T through diffusion and hexagon ring formation at the tube rim. |
| $P_C$ | (effective) carbon source pressure | 1.00* | | Pa | includes various carbon sources |
| $P_e$ | (effective) etching agent pressure | 1.00* | | Pa | includes various etching agents |
| | | | | | |
| $\lambda$ | $P_C$ multiplication factor | 2.39* | 5% | - | $=(1-\alpha)^{-1}$ |
| $s$ | $\Gamma_e$ multiplication factor | | | - | |
| $S_e$ | sensitivity to $k_e$ | | | - | |
| $S_g$ | sensitivity to $k_g$ | | | - | $S_e < 0$ |
| $S_{g/e}$ | dominance of $k_g$ in determining $\gamma_g$ | | | - | $=S_g+\zeta * S_e$ |
| $\zeta$ | weight coefficient | | | - | $\zeta<1$ is used,<br>since $\lvert S_e\rvert>\lvert S_g\rvert$ |
| | | | | | |
| $\omega_{label}$ | Peak frequency of a Raman mode at labels | | | $cm^{-1}$ | G-mode for s-SWCNTs, D-mode for m-SWCNTs |
| $\omega_0$ | Peak frequency of a Raman mode for $^{12}$CNT | | | $cm^{-1}$ | G-mode for s-SWCNTs, D-mode for m-SWCNTs |
| $\alpha$ | $^{12}$C ratio in isotope labels | | | - | Interested in the nanotube segments grown from $^{13}$C ethanol and $^{12}$C acetylene. |
| | | | | | |
| $n$ | chiral index | | | - | |
| $m$ | chiral index | | | - | |
| | | | | | |
| $T$ | Temperature of furnaces | | | °C | 800 for all experiments |

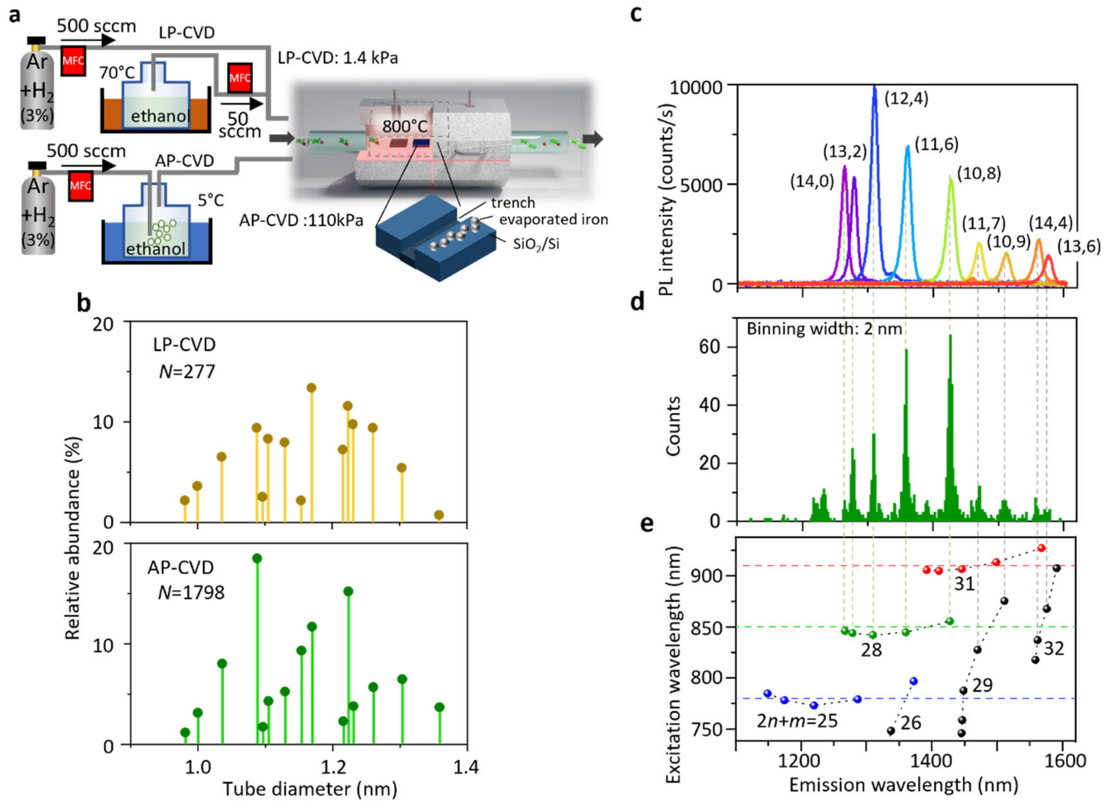


**Fig. S1 | Growth of air-suspended nanotubes and their photoluminescence measurements. a**, Schematic for the experimental setups for ethanol CVD at low pressure (LP) and atmospheric pressure (AP). In the LP-CVD, the ethanol tank is heated to 70°C to increase the vapor pressure and supplied at the controlled flow rate. In the AP-CVD, the ethanol tank is cooled to 5°C to lower the vapor pressure. **b**, Population of SWCNTs with each chirality (*n*,*m*) sorted by the diameter for the LP- (upper) and AP-CVD (lower). **c**, Typical PL spectra of individual nanotubes whose chirality can be assigned with an excitation wavelength of 850 nm. Among these chirality types, only those in a close resonant are included in the chirality distributions in (b) to avoid the bias caused by different absorption cross sections at a given excitation energy. **d**, Number distribution of peak position of PL emission spectra whose peak intensity is above the threshold (1000 counts/s) with the excitation wavelength of 850 nm. Excitation powers of 20 and 10 μW are used for the samples by LP-CVD and AP-CVD, respectively. **e**, Chirality map showing emission peak positions $E_{11}$ and absorption peak positions $E_{22}$. Chiral indices shown in blue, green, and red are included in the chirality distribution in (b).

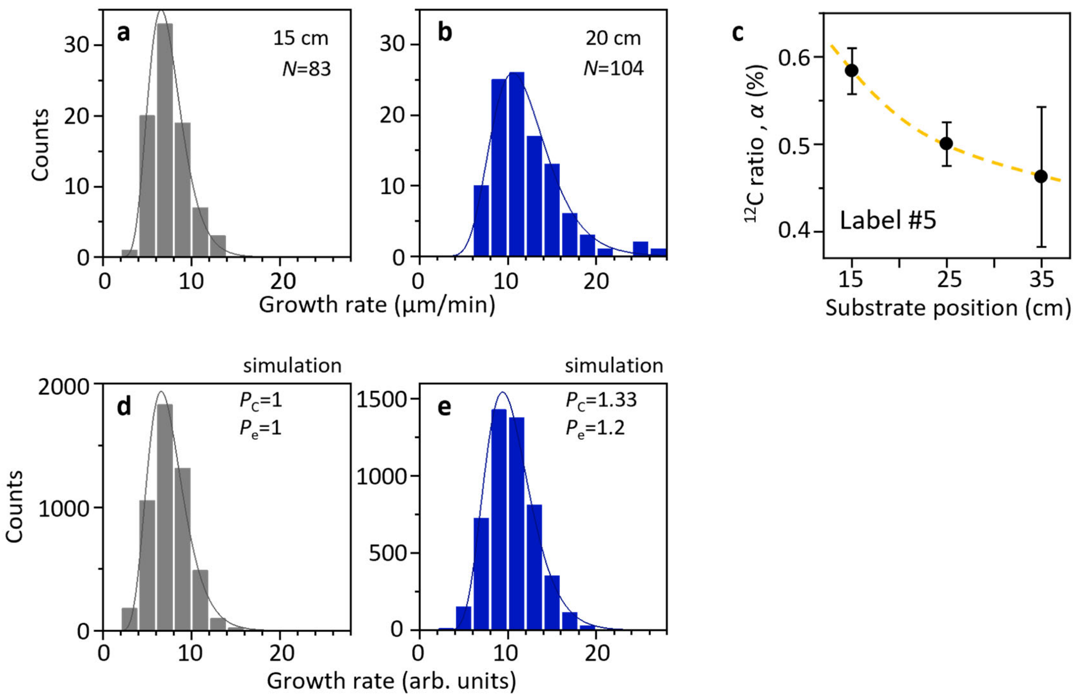


**Fig. S2 | Position-dependent growth rate studies by isotope labeling. a**,**b**, Experimental growth rate distributions obtained by the isotope labeling method[1] for the ethanol CVD without any additive gas than Ar and $H_2$ as a buffer gas. The positions of substrates are 15 and 20 cm from the upstream edge of the furnace for (a) and (b), respectively. **c**, Position-dependent fraction of $^{12}C$ in the nanotube parts grown from the mixture of $^{12}C_2H_2$ and $^{13}C_2H_5OH$ in the duplex labeling CVD. At the downstream of the furnace, more reactive hydrocarbon species are generated, and the relative contribution from $^{12}C$ acetylene becomes smaller. Error bars represent the 95% confidence interval. Dashed line is a guide for the eye. **d**,**e**, Simulated growth rate distributions with the parameters similar to those in Fig. 2d (d), and with the slightly modified $P_C$ and $P_e$, according to the result in (c) and the decomposition simulation in Fig. S3a (e). In the experiments, a few nanotubes have exceptionally large growth rates beyond the log-normal distribution, probably accounting for the presence of the outliers in Fig. 3h. They might originate from a different growth mode[5] or other catalyst from impurity.

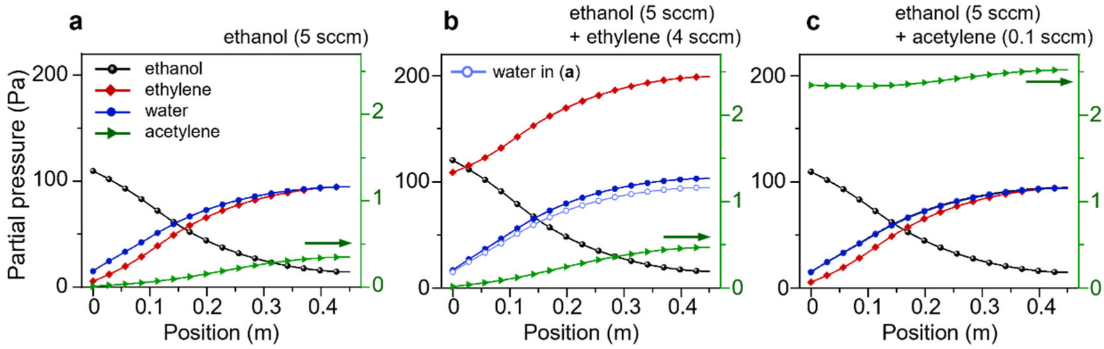


**Fig. S3 | Gas-phase decomposition simulation for ethanol flowing in the furnace.** Simulated partial pressures of major gas species as a function of position along the furnace. $Ar/H_2$ buffer gas is added to keep the total flow rate of 55 sccm for all cases. **a**, Ethanol (5 sccm) is supplied. **b**, Ethylene (4 sccm) is added to the condition in (a). **c**, Acetylene (0.1 sccm) is added to the condition in (a). In (b,c), the water pressure for the case (a) is shown for comparison. The upstream end of the electric furnace is taken as the origin. Total pressure is 1300 Pa, and the experimentally measured temperature profile along the furnace is used for the simulations. Ethanol (black spheres), ethylene (red diamonds), and water (blue circles) belong to the left-hand axis, while acetylene (green triangles) belongs to the right-hand axis. If ethylene is used as a growth modulator, a greater flow rate will be needed than the case of acetylene[3], and the addition of ethylene thus influences the generation of water, shifting $P_e$ as well as $P_C$. According to our previous study[6], $H_2$ does not work as an etching agent at 800°C that removes carbon from the catalyst and hence is not shown here, though we include $H_2$ in the simulations.

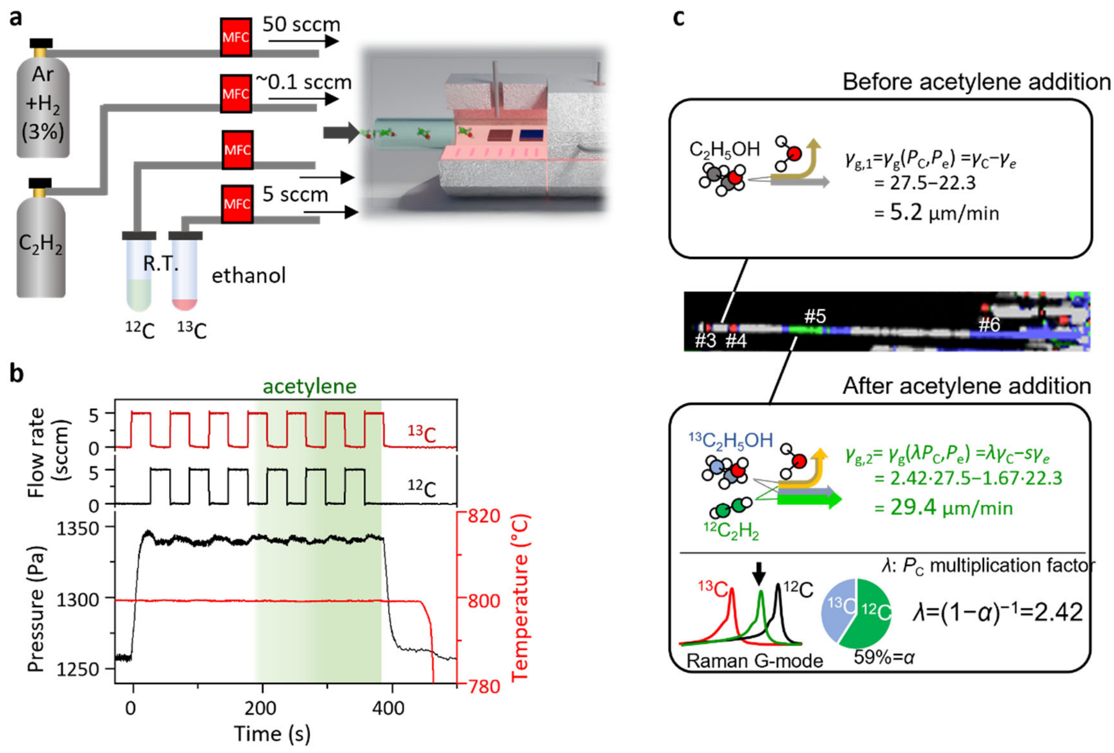


**Fig. S4 | Experimental conditions for the CVD growth with acetylene addition. a**, Schematic showing the CVD setup for the duplex labeling with isotope ethanol and acetylene. **b**, Measured parameters (flow rates, furnace temperature, and pressure) during the growth. Ethanol supply starts at 0 s. **c**, Schematic of "carbon bookkeeping" that breaks down the growth rates ($\gamma_{g,1}$, $\gamma_{g,2}$) into the carbon supply from ethanol/acetylene and the carbon removal from catalyst by water vapor. Growth rate breakdown is based on Eq. 4 and 5 in the main text, where $\lambda$ and $s$ are obtained from the Raman spectra (the inset of Fig. 2c) and the slope of the $\gamma_{g,1}$-$\gamma_{g,2}$ relationship (Fig. 2d), respectively. Raman mapping image in the middle is the same one as in Fig. 2a.

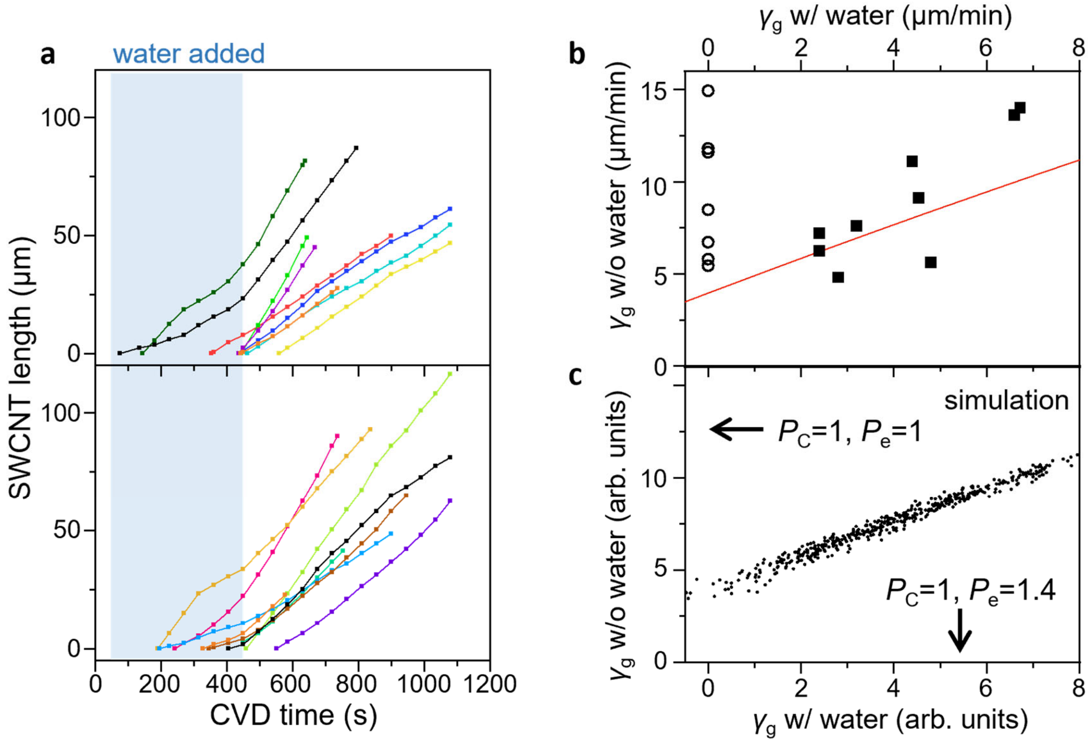


**Fig. S5 | Growth rate modulation by water vapor addition. a**, Growth curves of SWCNTs grown with the water-assisted ethanol CVD method. Water vapor with a flow rate of 1 sccm, which accounts for 24.6 Pa, is added to 5 sccm of ethanol 45–450 s after ethanol supply starts. Nanotube growth history is traced by the digital isotope coding method.[1] **b**, For the nanotubes that keep growing with and without water addition, growth rates before and after 450 s are plotted (black squares). For the nanotubes that initiate the growth at 450 s, growth rates without water addition are plotted (open circles). We suspect the latter plots include the nanotubes that go through shrinkage due to the added water, as well as those which happens to start nucleation at ~450 s. Solid line represents the deterministic relationship derived from the kinetic model. **c**, Simulated growth rate relationship that corresponds to the experiments in (a,b). From the thermal decomposition simulation (Fig. S3) and the flow rate (1 sccm), the effective $P_e$ with water addition is expected to become 1.4× larger, although we stress that the actual multiplication factor of $P_e$ is experimentally unknown.

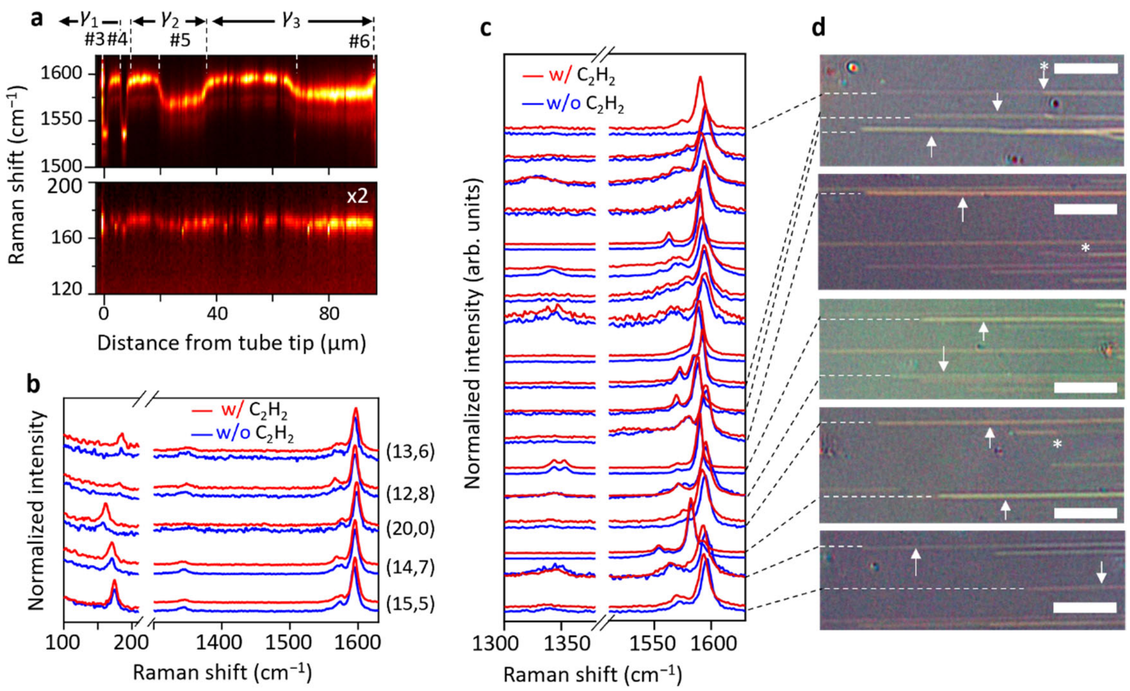


**Fig. S6 | Optical comparison of the nanotubes grown with and without acetylene. a**, Raman spectra along the entire length of a typical SWCNT. **b**, Raman spectra (G, D, and radial breathing modes (RBM)) of five nanotubes grown from ethanol only (blue) and from the mixture of acetylene (red), showing no significant difference. **c**, Raman spectra obtained in the other set of experiments and **d**, corresponding optical images of the nanotubes (see Supplementary Note 3). White arrows indicate the junction at which the acetylene addition starts. In a rare case, the tube chirality changes as indicated by asterisks. Scale bars are 5 µm.

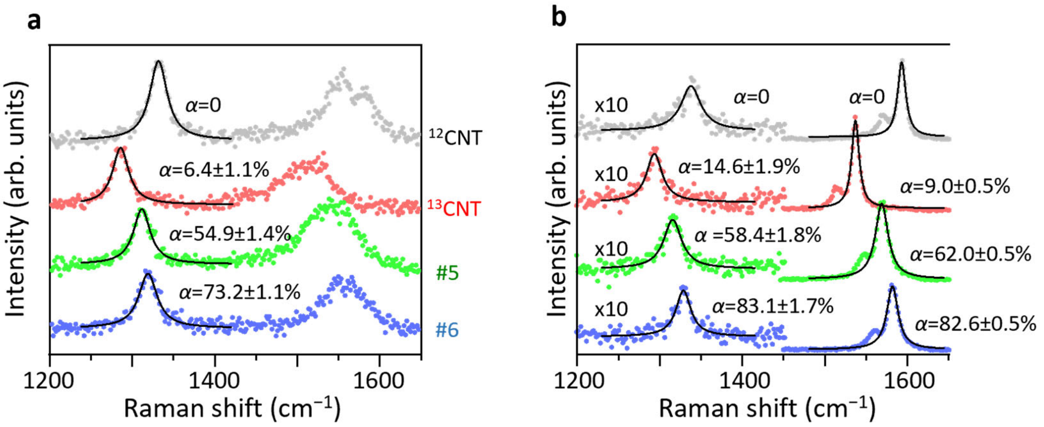


**Fig. S7 | Determination of isotope ratios from Raman spectra. a**, Raman spectra of a typical metallic nanotube measured at four characteristic regions ($^{12}$CNT, $^{13}$CNT, label #5 and #6). Black lines represent the Lorentzian fitting of D-band. The $^{12}$C ratio $\alpha$ is calculated from the relation $\omega_{\mathrm{label}} = \omega_0\sqrt{12.01/(12.01\alpha + 12.99(1-\alpha))}$, where $\omega_{\mathrm{label}}$ and $\omega_0$ represent the G- (or D-) peak frequency at isotope label parts and that of $^{12}$C-derived nanotubes, respectively. Note that average atomic weights of our $^{12}$C acetylene and $^{13}$C ethanol are 12.01 and 12.99, respectively. **b**, Raman spectra of a typical semiconducting nanotube. The $^{12}$C fraction $\alpha$ in each part is compared between the G-band basis and the D-band basis.

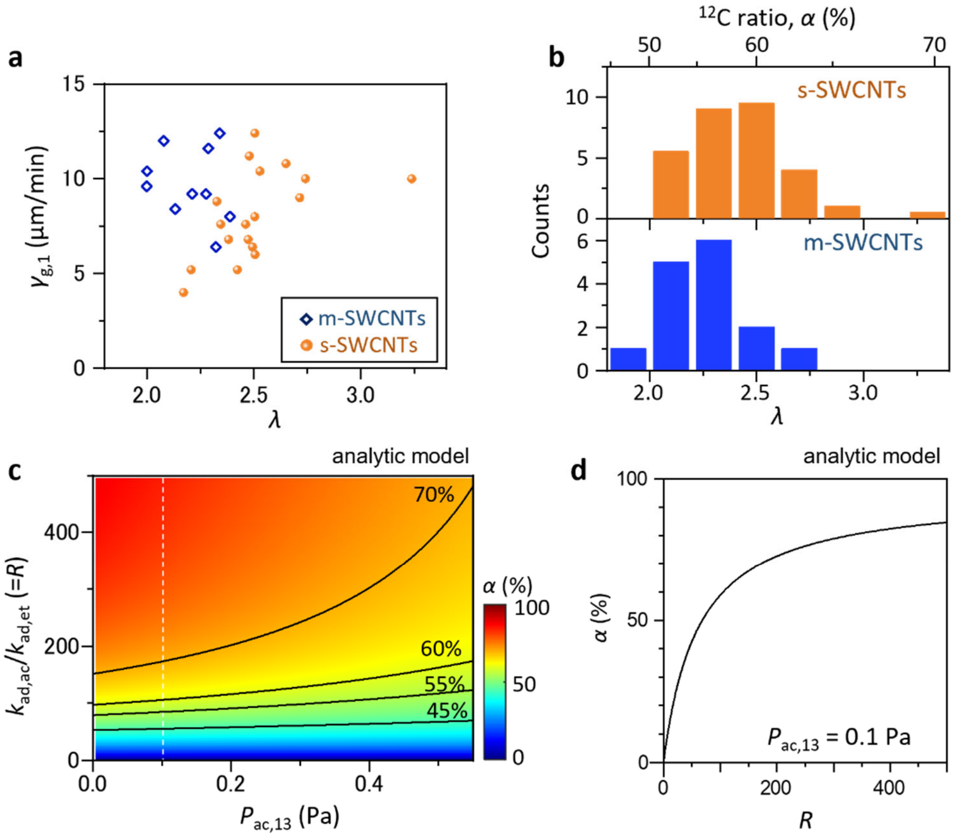


**Fig. S8 | Tube-to-tube variation of adsorption efficiency of carbon sources. a**, $\lambda$ versus growth rate $\gamma_{g,1}$ for s- and m-SWNCTs. **b**, Distributions of $\lambda$ for s- and m-SWCNTs. A larger number of nanotubes are counted than in (a) because $\gamma_{g,1}$ does not need to be defined. **c**, Calculated $^{12}$C ratio $\alpha$ in the isotope label from the mixture of $^{13}$C ethanol and $^{12}$C acetylene as a function of the partial pressure of acetylene from ethanol decomposition and $k_{ad,ac}/k_{ad,at}$, where $k_{ad,ac}$ and $k_{ad,et}$ represent adsorption efficiencies for acetylene and the mixture of ethanol/ethylene, respectively. Since the gas composition is the same at the same location of the furnace, x-axis should be fixed for all nanotubes, but y-axis should vary tube to tube. **d**, $R$ versus $\alpha$ when the acetylene from ethanol accounts for 0.1 Pa is assumed (see Fig. S3). $\alpha$=55 and 60% corresponds to $k_{ad,ac}/k_{ad,et}$ = 85 and 106, respectively. Overall, these results tell us that ethanol is more easily adsorbed on the catalyst connected to m-SWCNTs.

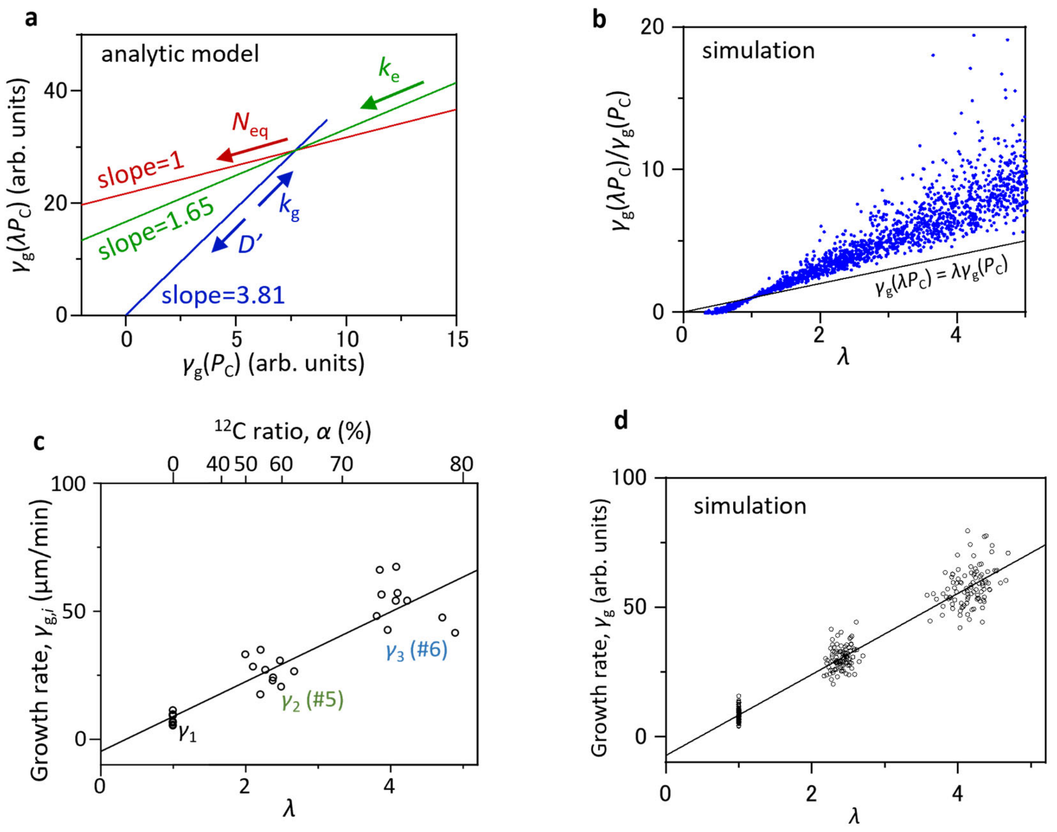


**Fig. S9 | Model-based growth rate change due to increased carbon supply.** **a**, Analytical relationships between $\gamma_g(P_C)$ and $\gamma_g(\lambda P_C)$, assuming $N_{eq}$, $k_e$, or $k_g$ (or $D'$) to be an intervening parameter. $\lambda$=2.39. When $k_g$ and $N_{eq}$ are eliminated from the equations for $\gamma_g(P_C)$ and $\gamma_g(\lambda P_C)$, Eq. S2 and S3 are obtained. **b**, Simulated relationship between $\lambda$ and $\gamma_g(\lambda P_C)/\gamma_g(P_C)$ for uniformly distributed $\lambda$, which corresponds to the experimental results in Fig. 2c. **c**, Experimental growth rates as a function of $\lambda$ for $\gamma_{g,i}$ ($i$=1–3) and **d**, corresponding simulated growth rates with $\lambda = 1$, $\bar{\lambda} = 2.39, 4.15$.

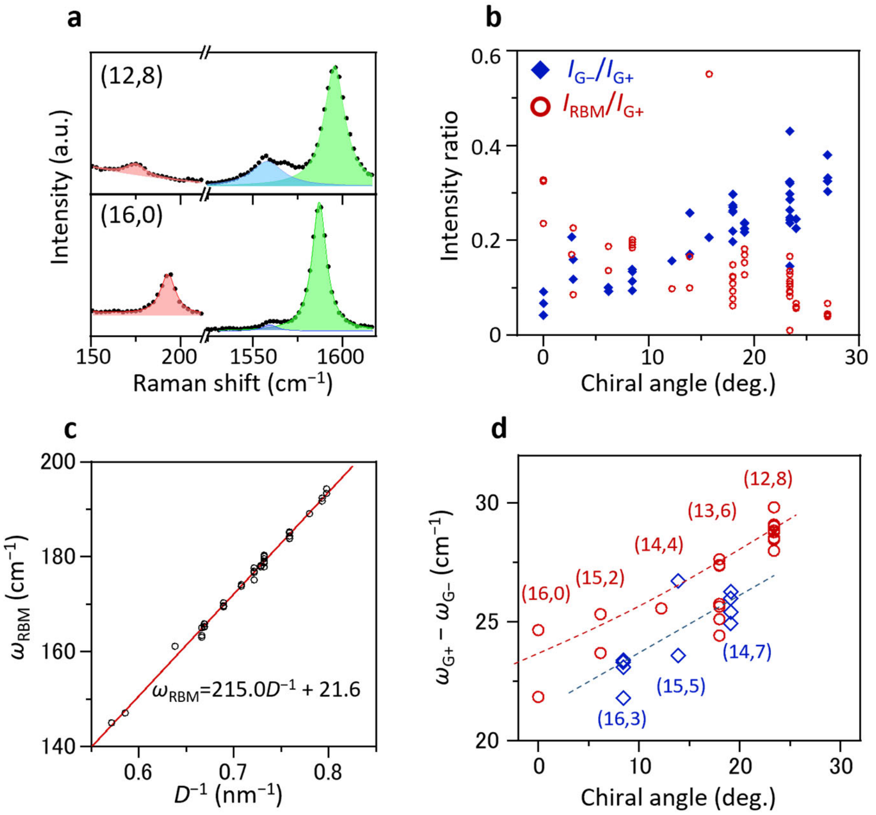


**Fig. S10 | Chirality assignment using multiple characteristics of Raman spectra.** **a**, Raman spectra and its peak fits for $G^+$, $G^-$, and RBM for intensity comparison. **b**, The intensity ratio, $I_{G-}/I_{G+}$ (blue) and $I_{RBM}/I_{G+}$ (red), plotted as a function of the chiral angle. **c**, Relationship between diameter and RBM peak position. **d**, Distance between the peak positions of $G^+$ and $G^-$ modes, which depends on the diameter and chiral angle. Dashed lines are guides for the eye. All Raman spectra in Fig. S10 are measured on $SiO_2$/Si substrates excited with a laser wavelength of 532 nm.

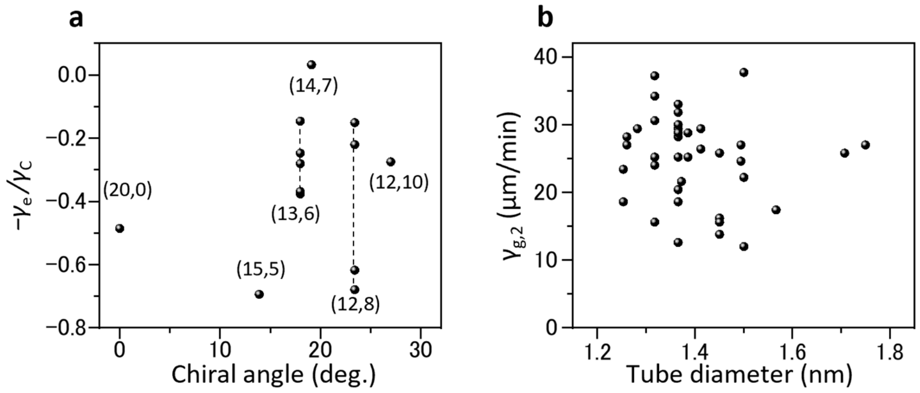


**Fig. S11 | Chirality dependence of carbon removal effects and growth rate.** **a**, Chiral angle dependence of $-\gamma_e/\gamma_C$ for the plots shown in Fig. 2e. **b**, Diameter dependence of the growth rate $\gamma_{g,2}$ after the acetylene addition for the data shown in Fig. 3a.

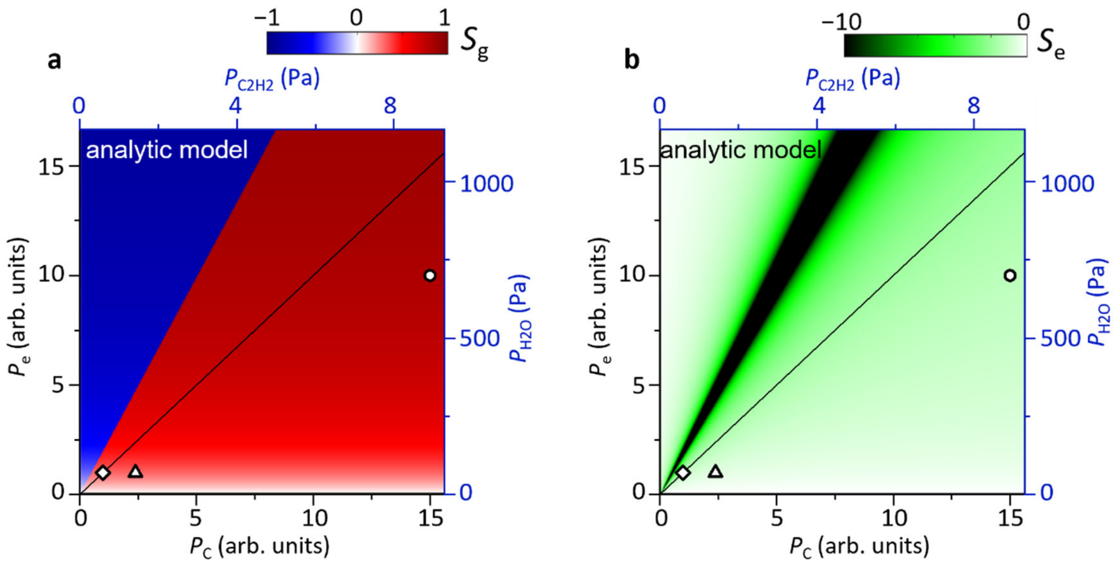


**Fig. S12 | Sensitivity of growth rate to $k_g$ and $k_e$. a**,**b**, Sensitivity of the growth rate to $k_g$ ($S_g$) and $k_e$ ($S_e$) change as a function of a function of $P_C$ and $P_e$. The upper axis shows the equivalent pressure of acetylene, judging from the observation that 0.077 sccm of acetylene (~1.87 Pa) accounts for the increase in $P_C$ by 4.15-fold. The right axis shows the that of water based on the decomposition simulation using the COMSOL software.

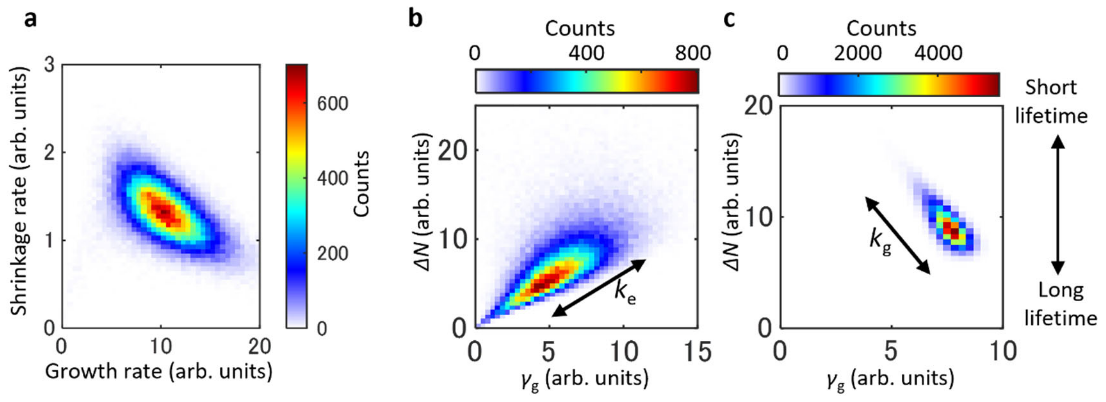


**Fig. S13 | Correlation between growth rate, shrinking rate, and lifetime. a**, Relationship between the growth rate with ethanol supply and the carbon removal rate with water supply in the simulations that emulate the experimental conditions in the previous study[6]. Both $P_C$ and $P_e$ are 1 for the growth, whereas $P_C$ = 0 and $P_e$ = 0.1 for the shrinkage. In this simulation, the variations of $k_g$, $k_e$, and $A$ are 30, 20, and 10%, respectively. The $k_e$ dependence of growth and shrinkage results in the negative correlation, whereas the $k_g$ dependence contributes to the position correlation in the distribution. **b**,**c**, Distribution of growth rates $\gamma_g$ and supersaturation $\Delta N$ when $k_g$ and $k_e$ have a variation of 20% (b), and when only $k_g$ has a relative standard deviation of 20% with a fixed $k_e$. In general, a large $\Delta N$ should lead to a short catalyst lifetime due to encapsulation by carbon shells.

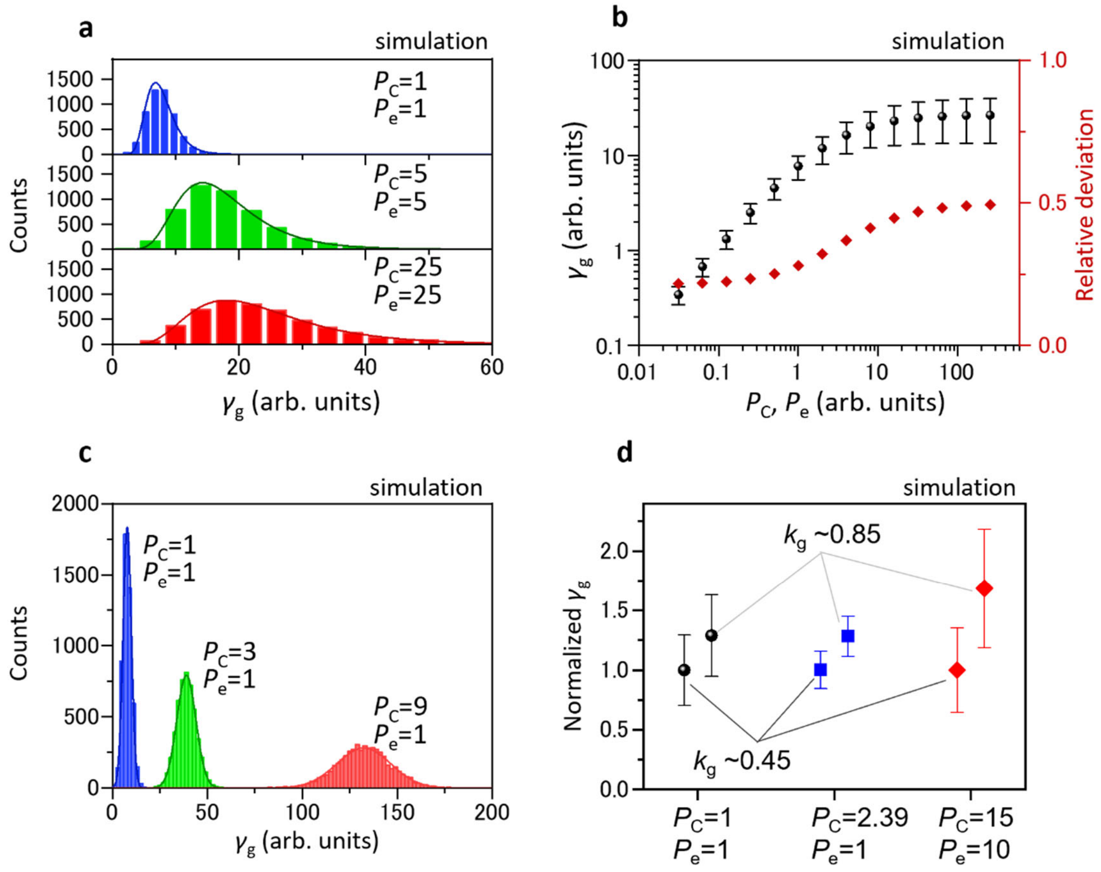


**Fig. S14 | Distribution of growth rate depending on the pressures of carbon sources and etching agents. a**, Simulated growth rate distributions with the $P_C/P_e$ ratio kept constant, which correspond to the pressure dependence in the ethanol CVD. All the distributions are fitted well with a log-normal function. Hence, under the growth condition along this solid line in Fig. 4, the growth rate distribution rather follows a log-normal distribution, in good agreement with a recent study on growth kinetics of individual nanotubes[7]. **b**, Average growth rate and its standard deviation (error bars) as a function of the ethanol partial pressure, to which $P_C$ and $P_e$ are proportional. The growth rate saturates at the high-pressure limit due to the balancing between carbon supply and removal, while the relative scatter of growth rates should increase with the pressure increase. **c**, Simulated growth rate distributions at different $P_C$ levels with $P_e$ being unchanged. All the distribution can be fitted by a normal distribution. **d**, Average growth rate $\gamma_g$ normalized by that with $0.4 \leq k_g < 0.5$ for three different conditions, corresponding to the data shown in Fig. 3d and e. Error bars represent the standard deviation.

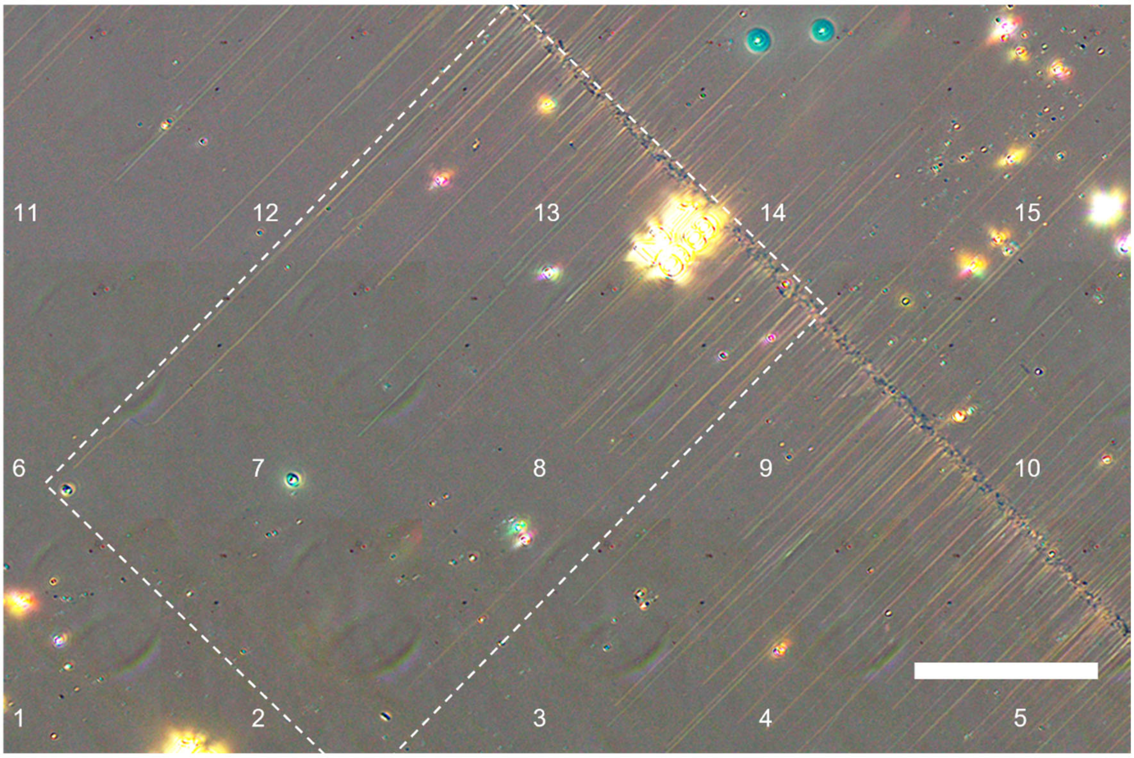


**Fig. S15 | Quasi-true color optical image in a large area.** Representative fifteen images are obtained with the contrast enhancement by crossed polarizers and combined to form a single large image. The dashed rectangle represents the area whose Raman mapping is shown in Fig. 2b. The color of images is based on the RGB values acquired by a camera but processed in a manner described in Supplementary Note 3. The numbers 1–15 in the figure indicate different shots of the camera. Scale bar is 50 µm.

**Table S2 | CVD conditions used for the main results.** For all the cases, iron is used as the catalyst that is deposited by thermal or electron-beam evaporation with the nominal thickness of 0.1 nm. In the isotope labeling experiment in Fig. 3f–h, the isotope ratio of ethanol is gradually changed, unlike the rapid switching for the experiment for Fig. 2 because gas diffusion may disable the discrete isotope switching at the reduce gas velocity. †The initial pressure of ~600 Pa includes Ar/$H_2$ used for the reduction of catalyst particles prior to the synthesis step.

| Condition | Gas | Flow rate (sccm) | Temperature (°C) | Total pressure (Pa) | Growth time (s) | Position (cm) | Quartz tube diameter (mm) |
|---|---|---|---|---|---|---|---|
| Fig. 1b | Ar | 485 | 800 | 1400 | 1200 | 20 | 26 |
| | $H_2$ | 15 | | | | | |
| | Ethanol | 50 | | | | | |
| Fig. 1c | Ar | 485 | 800 | $110\times10^3$ | 60 (w/ ethanol) +300 (w/o ethanol) | 45 | 26 |
| | $H_2$ | 15 | | | | | |
| | Ethanol | bubbling (5°C) | | | | | |
| Fig. 2a | Ar | 48.5 | 800 | 1300 | 195 (w/o acetylene) +195 (w/ acetylene) | 15 (25,35) | 26 |
| | $H_2$ | 1.5 | | | | | |
| | Ethanol | 5 | | | | | |
| | Acetylene | 0.077 (0.092) | | | | | |
| Fig. 3h | Ethanol | 5 | 800 | 600–1200† | 180 (w/ ethanol) +300 (w/o ethanol) | 25 | 26 |

**Table S3 | Average growth rates and related values**. Growth rates before and after the acetylene addition ($\gamma_{g,1}$ and $\gamma_{g,2}$, respectively) for semiconducting and metallic SWCNTs. Other characteristic values appearing in bookkeeping of carbon atoms during the growth ($\gamma_C$, $\gamma_e/\gamma_C$, and $\alpha$). In total, the catalyst particles connected to m-SWCNTs adsorb and dissociate ethanol and ethylene more actively than those connected to s-SWCNTs. At the same time, adsorbed carbon atoms on the catalyst connected to m-SWCNTs are easily removed.

| | **Semiconducting SWCNTs Average, s.d. (μm/min)** | | | | **Metallic SWCNTs Average, s.d. (μm/min)** | | | |
|---|---|---|---|---|---|---|---|---|
| $\gamma_{g,1}$ | 8.12 | ± | 2.35 | μm/min | 9.72 | ± | 1.90 | μm/min |
| $\gamma_{g,2}$ | 27.83 | ± | 6.61 | μm/min | 31.68 | ± | 5.31 | μm/min |
| $\gamma_C$ | 17.28 | ± | 10.32 | μm/min | 32.20 | ± | 5.34 | μm/min |
| $\gamma_e/\gamma_C$ | 0.47 | ± | 0.24 | | 0.68 | ± | 0.10 | |
| $\alpha$ | 0.60 | ± | 0.03 | | 0.54 | ± | 0.03 | |

**Supplementary information**

## References


1. Otsuka, K. *et al.* Digital Isotope Coding to Trace the Growth Process of Individual Single-Walled Carbon Nanotubes. *ACS Nano* **12**, 3994–4001 (2018).

2. Marinov, N. M. Kinetic Model for High Temperature Ethanol Oxidation. *Int. J. Chem. Kinet.* **31**, 183–220 (1999).

3. Xiang, R., Einarsson, E., Okawa, J., Miyauchi, Y. & Maruyama, S. Acetylene-accelerated alcohol catalytic chemical vapor deposition growth of vertically aligned single-walled carbon nanotubes. *J. Phys. Chem. C* **113**, 7511–7515 (2009).

4. Liu, K. *et al.* High-throughput optical imaging and spectroscopy of individual carbon nanotubes in devices. *Nat. Nanotechnol.* **8**, 917–922 (2013).

5. He, M. *et al.* Linking growth mode to lengths of single-walled carbon nanotubes. *Carbon* **113**, 231–236 (2017).

6. Koyano, B. *et al.* Regrowth and catalytic etching of individual single-walled carbon nanotubes studied by isotope labeling and growth interruption. *Carbon* **155**, 635–642 (2019).

7. Pimonov, V. *et al.* Dynamic Instability of Individual Carbon Nanotube Growth Revealed by In Situ Homodyne Polarization Microscopy. *Nano Lett.* **21**, 8495–8502 (2021).
